# Supplementary material for: Synergistic Offline-Online Control Synthesis via Local Gaussian Process Regression
Source: arXiv:2110.05525 source file (2022-03-08)
Supplement: Supplementary file 1 [file 99-appendix.tex]

% appendix.tex
\noindent
Appendix goes here ...
